# Supplementary material for: Blocks as geographic discontinuities: The effect of polling place assignment on voting
Source: arXiv:2105.01728 source file (2021-05-04)
Supplement: Supplementary file 1 [file additional_figures.tex]

\subsection{Additional Figures}
\label{sec:additional}
In \figref{diff_distances} we show the effect of relative distance for all blocks where the additional distance traveled by the treatment group ranges from 0 to more than 2 miles.  This figure also displays the average distance traveled by the voters on the closer block face, conditioned on a given relative distance. When we include all voters we see that the average distance is quite small and the effect of relative distance is around 2 \%. However, when we restrict our attention to those voters who live on a block with a relatively large difference between the distances traveled by the close and far block faces they tend to be live farther on average than the overall population. Thus while we see a more pronounced effected of relative distance for this group, this might be attributable to other characteristics of these voters which differentiate them from the rest. For example, they tend to be more rural.  

\begin{figure}[H]
\begin{center}
    \includegraphics[width=.75\columnwidth]{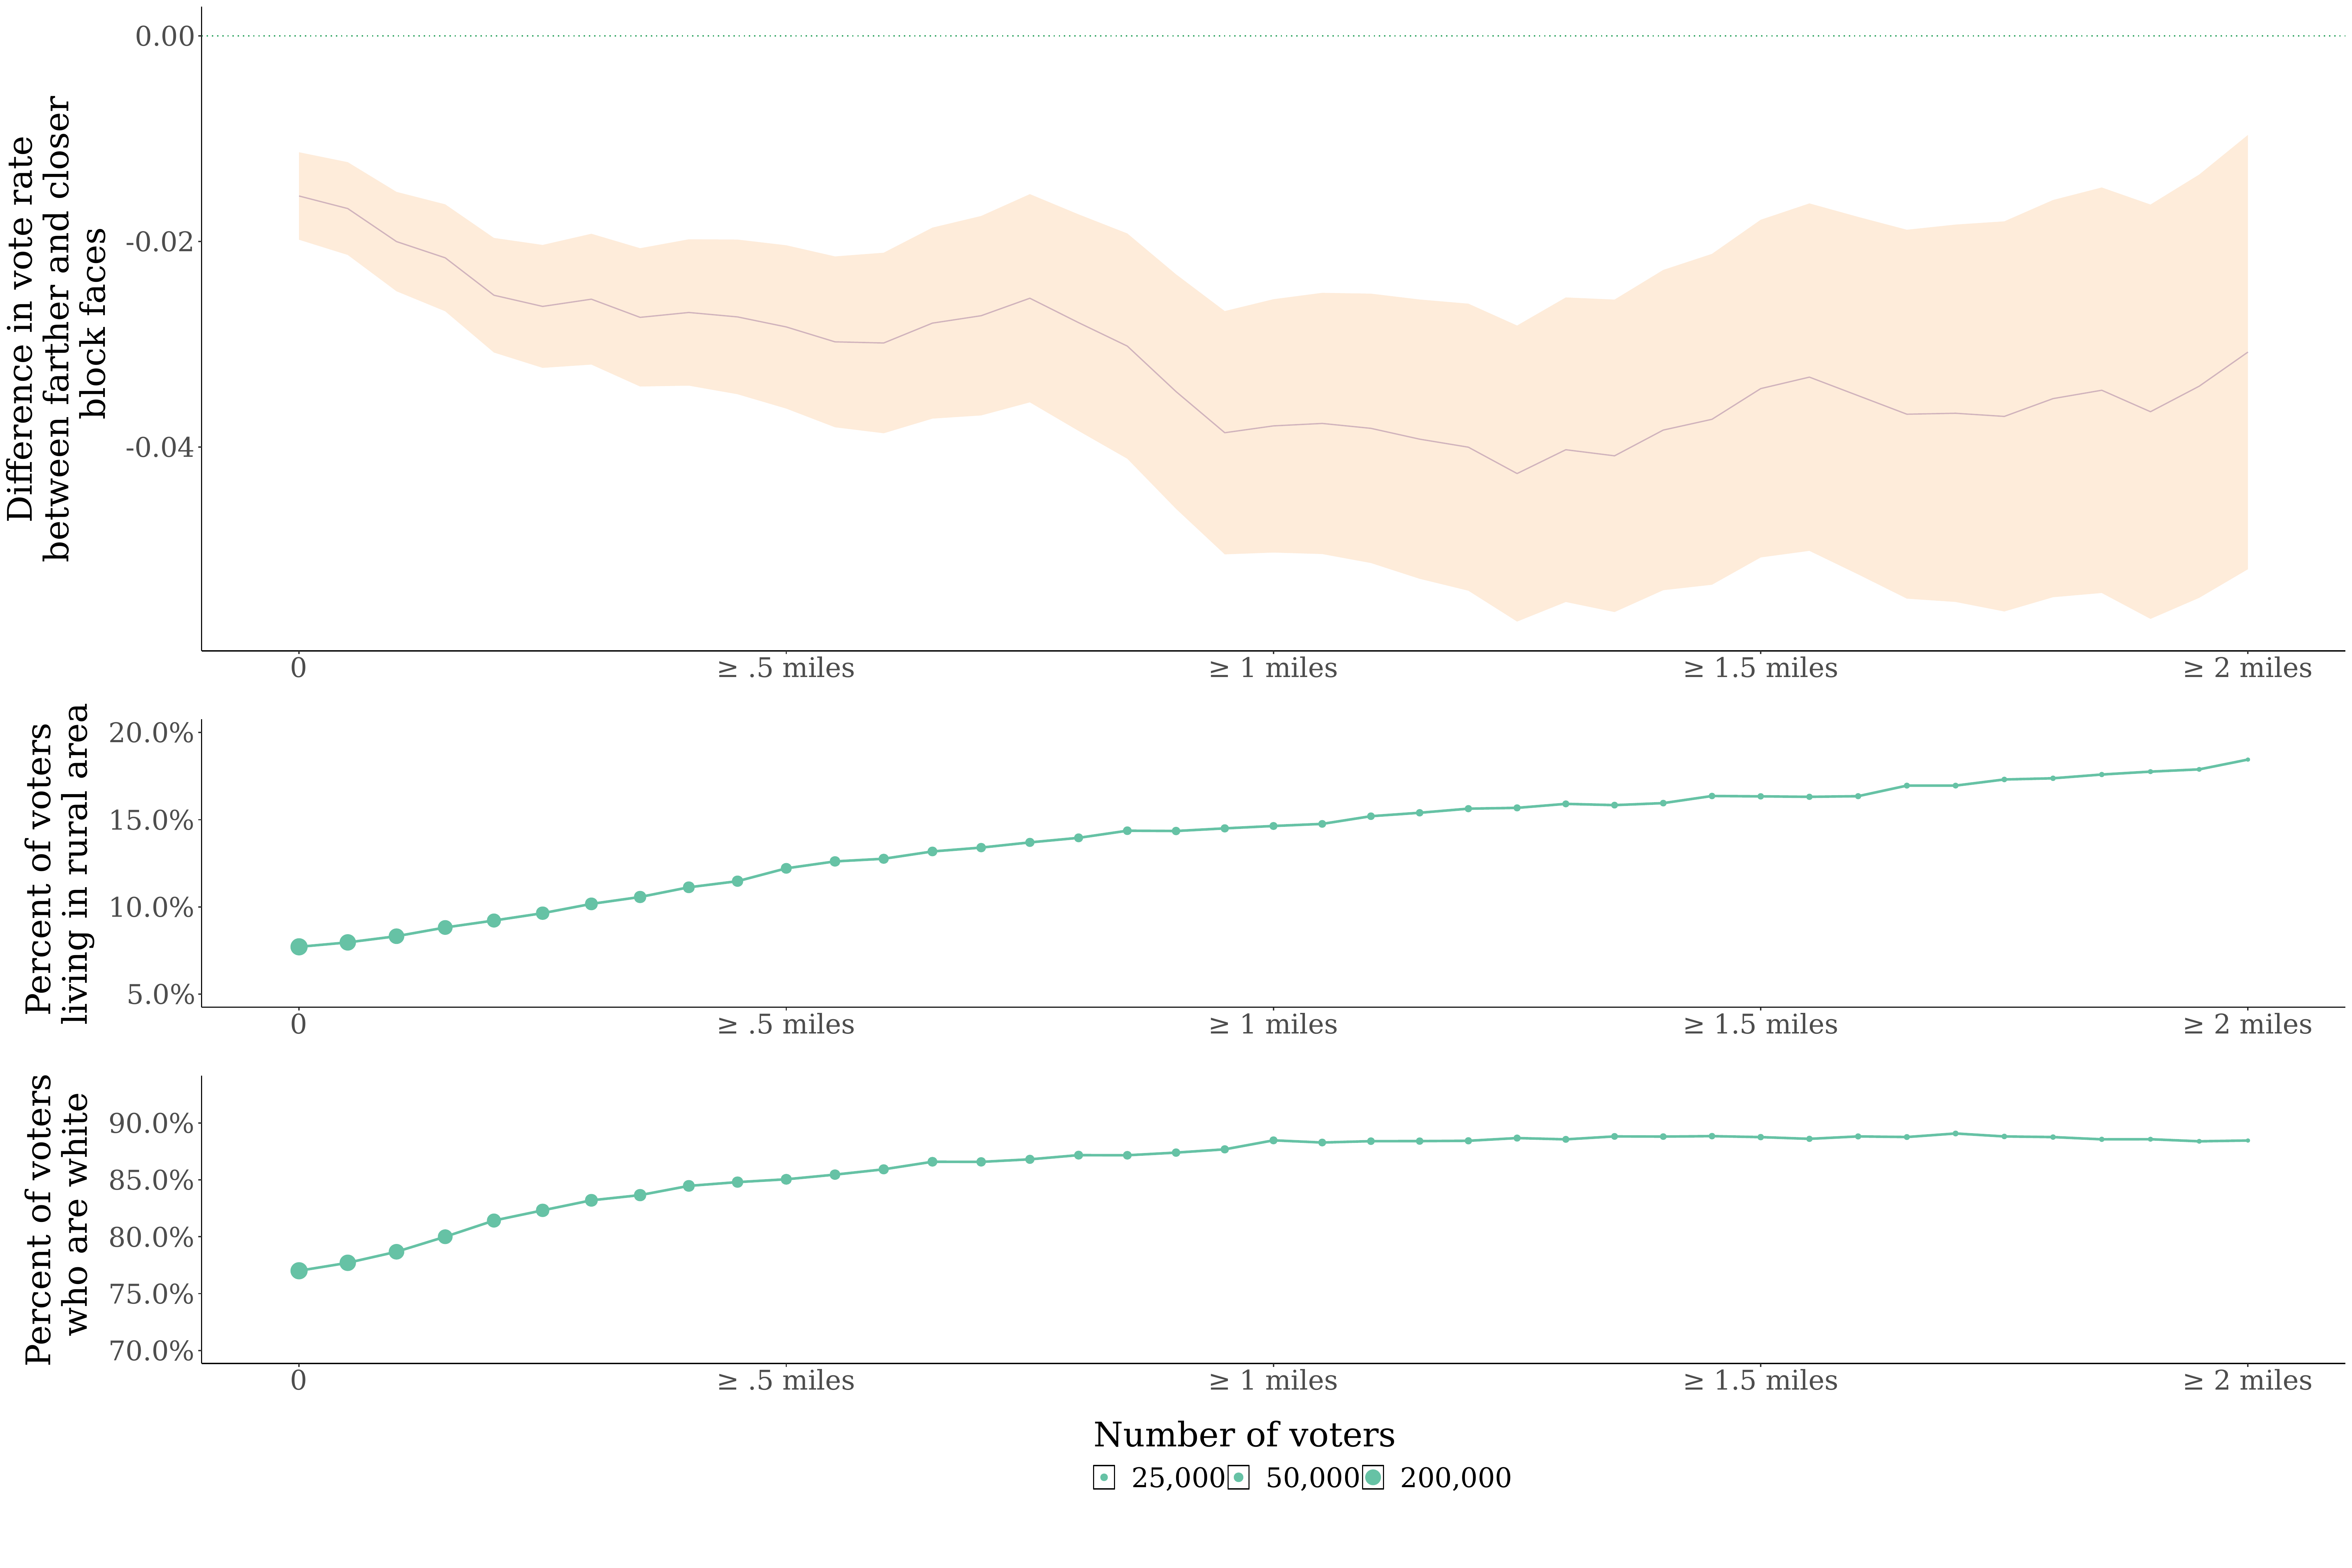}
    \caption{As the difference in distance between the closer and farther block faces grows, so does the effect of distance. However, the population also changes with distance.\label{diff_distances}  }  
   \end{center}
\end{figure}

The remainder of this sections show balance plots comparing the characteristics of registrants in a treatment groups and control group from our analyses. Each point is the difference between the proportion of registrants with a given characteristic in treatment and the proportion of registrants with this characteristic in control, divided by the proportion of registrants with a given characteristic in control. The size of each point is scaled by the number of registrants in the control group, where larger points represent groups with more registrants. We first present these graphs for the relative distance analysis, in which the treatment group is comprised of those registrants on the side of the block that is relatively further from the polling location. Then we present graphs for the shocks analysis, in which the treatment group is comprised of those registrants who experience a change in polling location. The difference between the proportion of registrants with a given characteristic in the treatment group relative to the control group is close to zero for the most common characteristics. For less common characteristics the difference can be greater, especially in the shocks analysis because the sample size is smaller.

\begin{figure}[H]

\centering
\resizebox{.7\linewidth}{!}{
    \includegraphics[ width=.99\columnwidth]{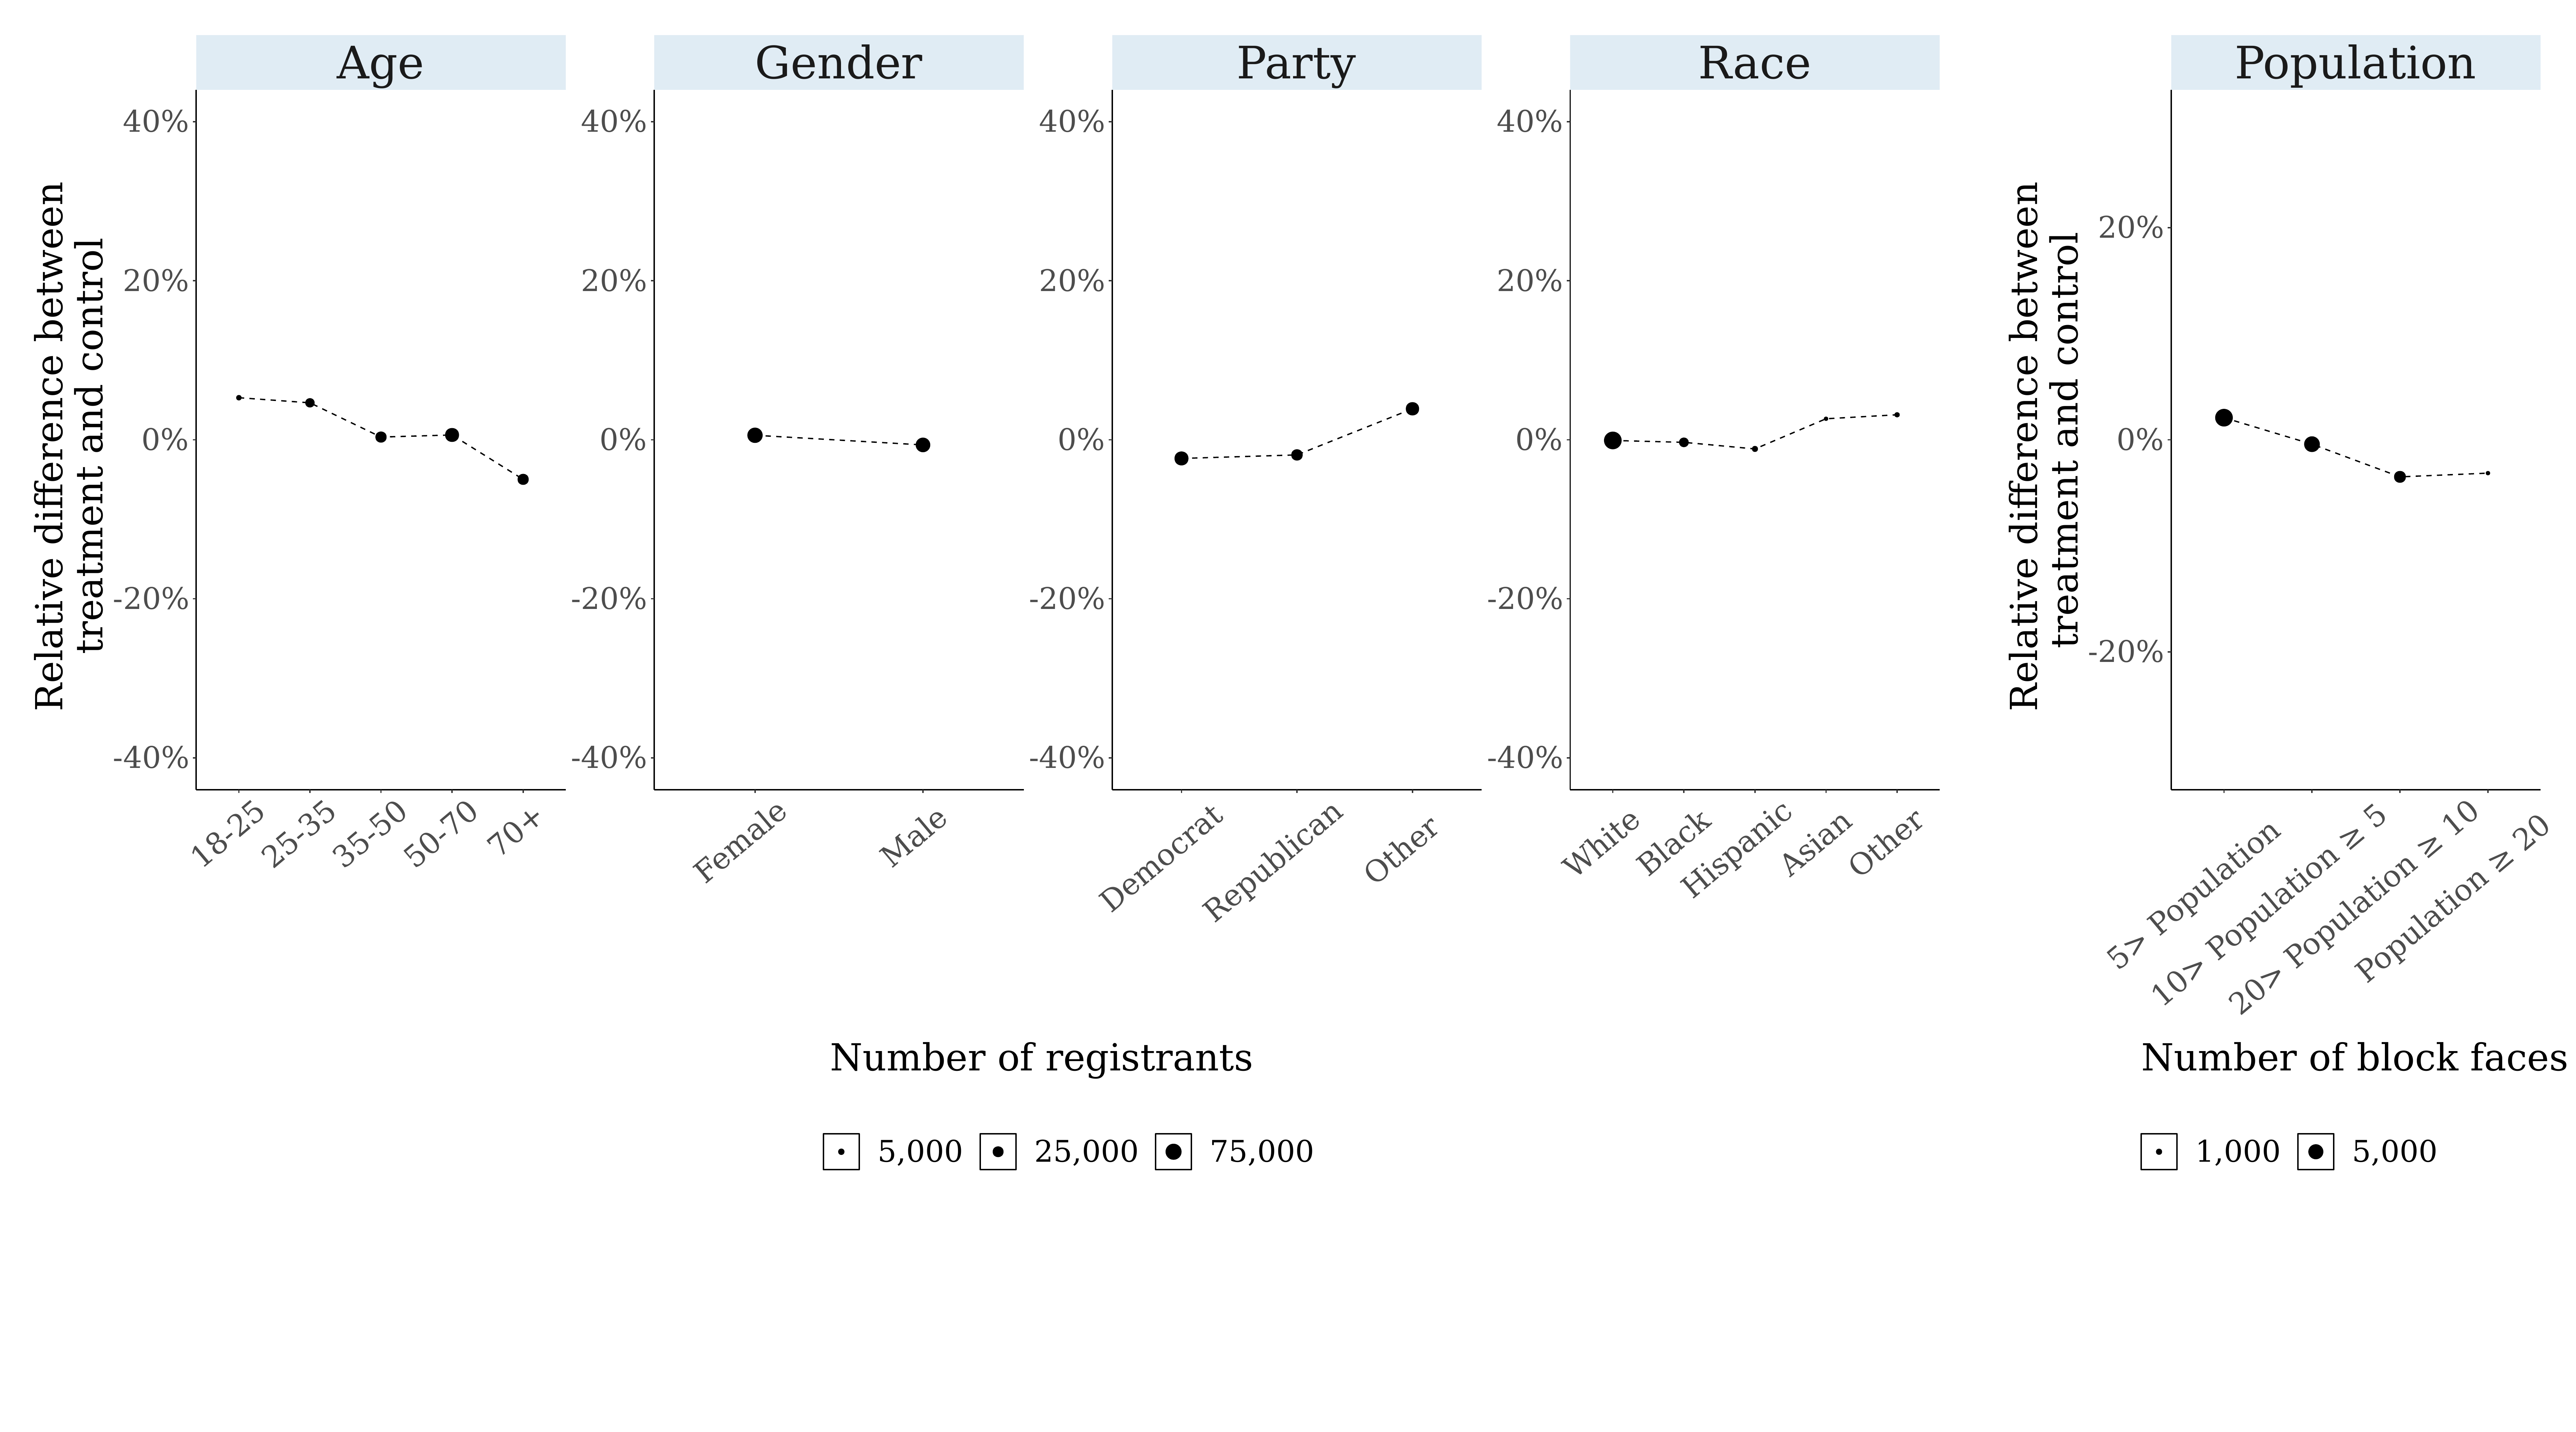}}
    \caption{We see the age, gender, modeled partisanship, modeled race of \units{}, as well as indicators representing that the total number of \units{} are similar on either block face. (Distance)
    } 
    \label{bp_distance}
    
\end{figure}

\begin{figure}[H]\centering
\resizebox{.4\linewidth}{!}{
    \includegraphics[width=.99\columnwidth]{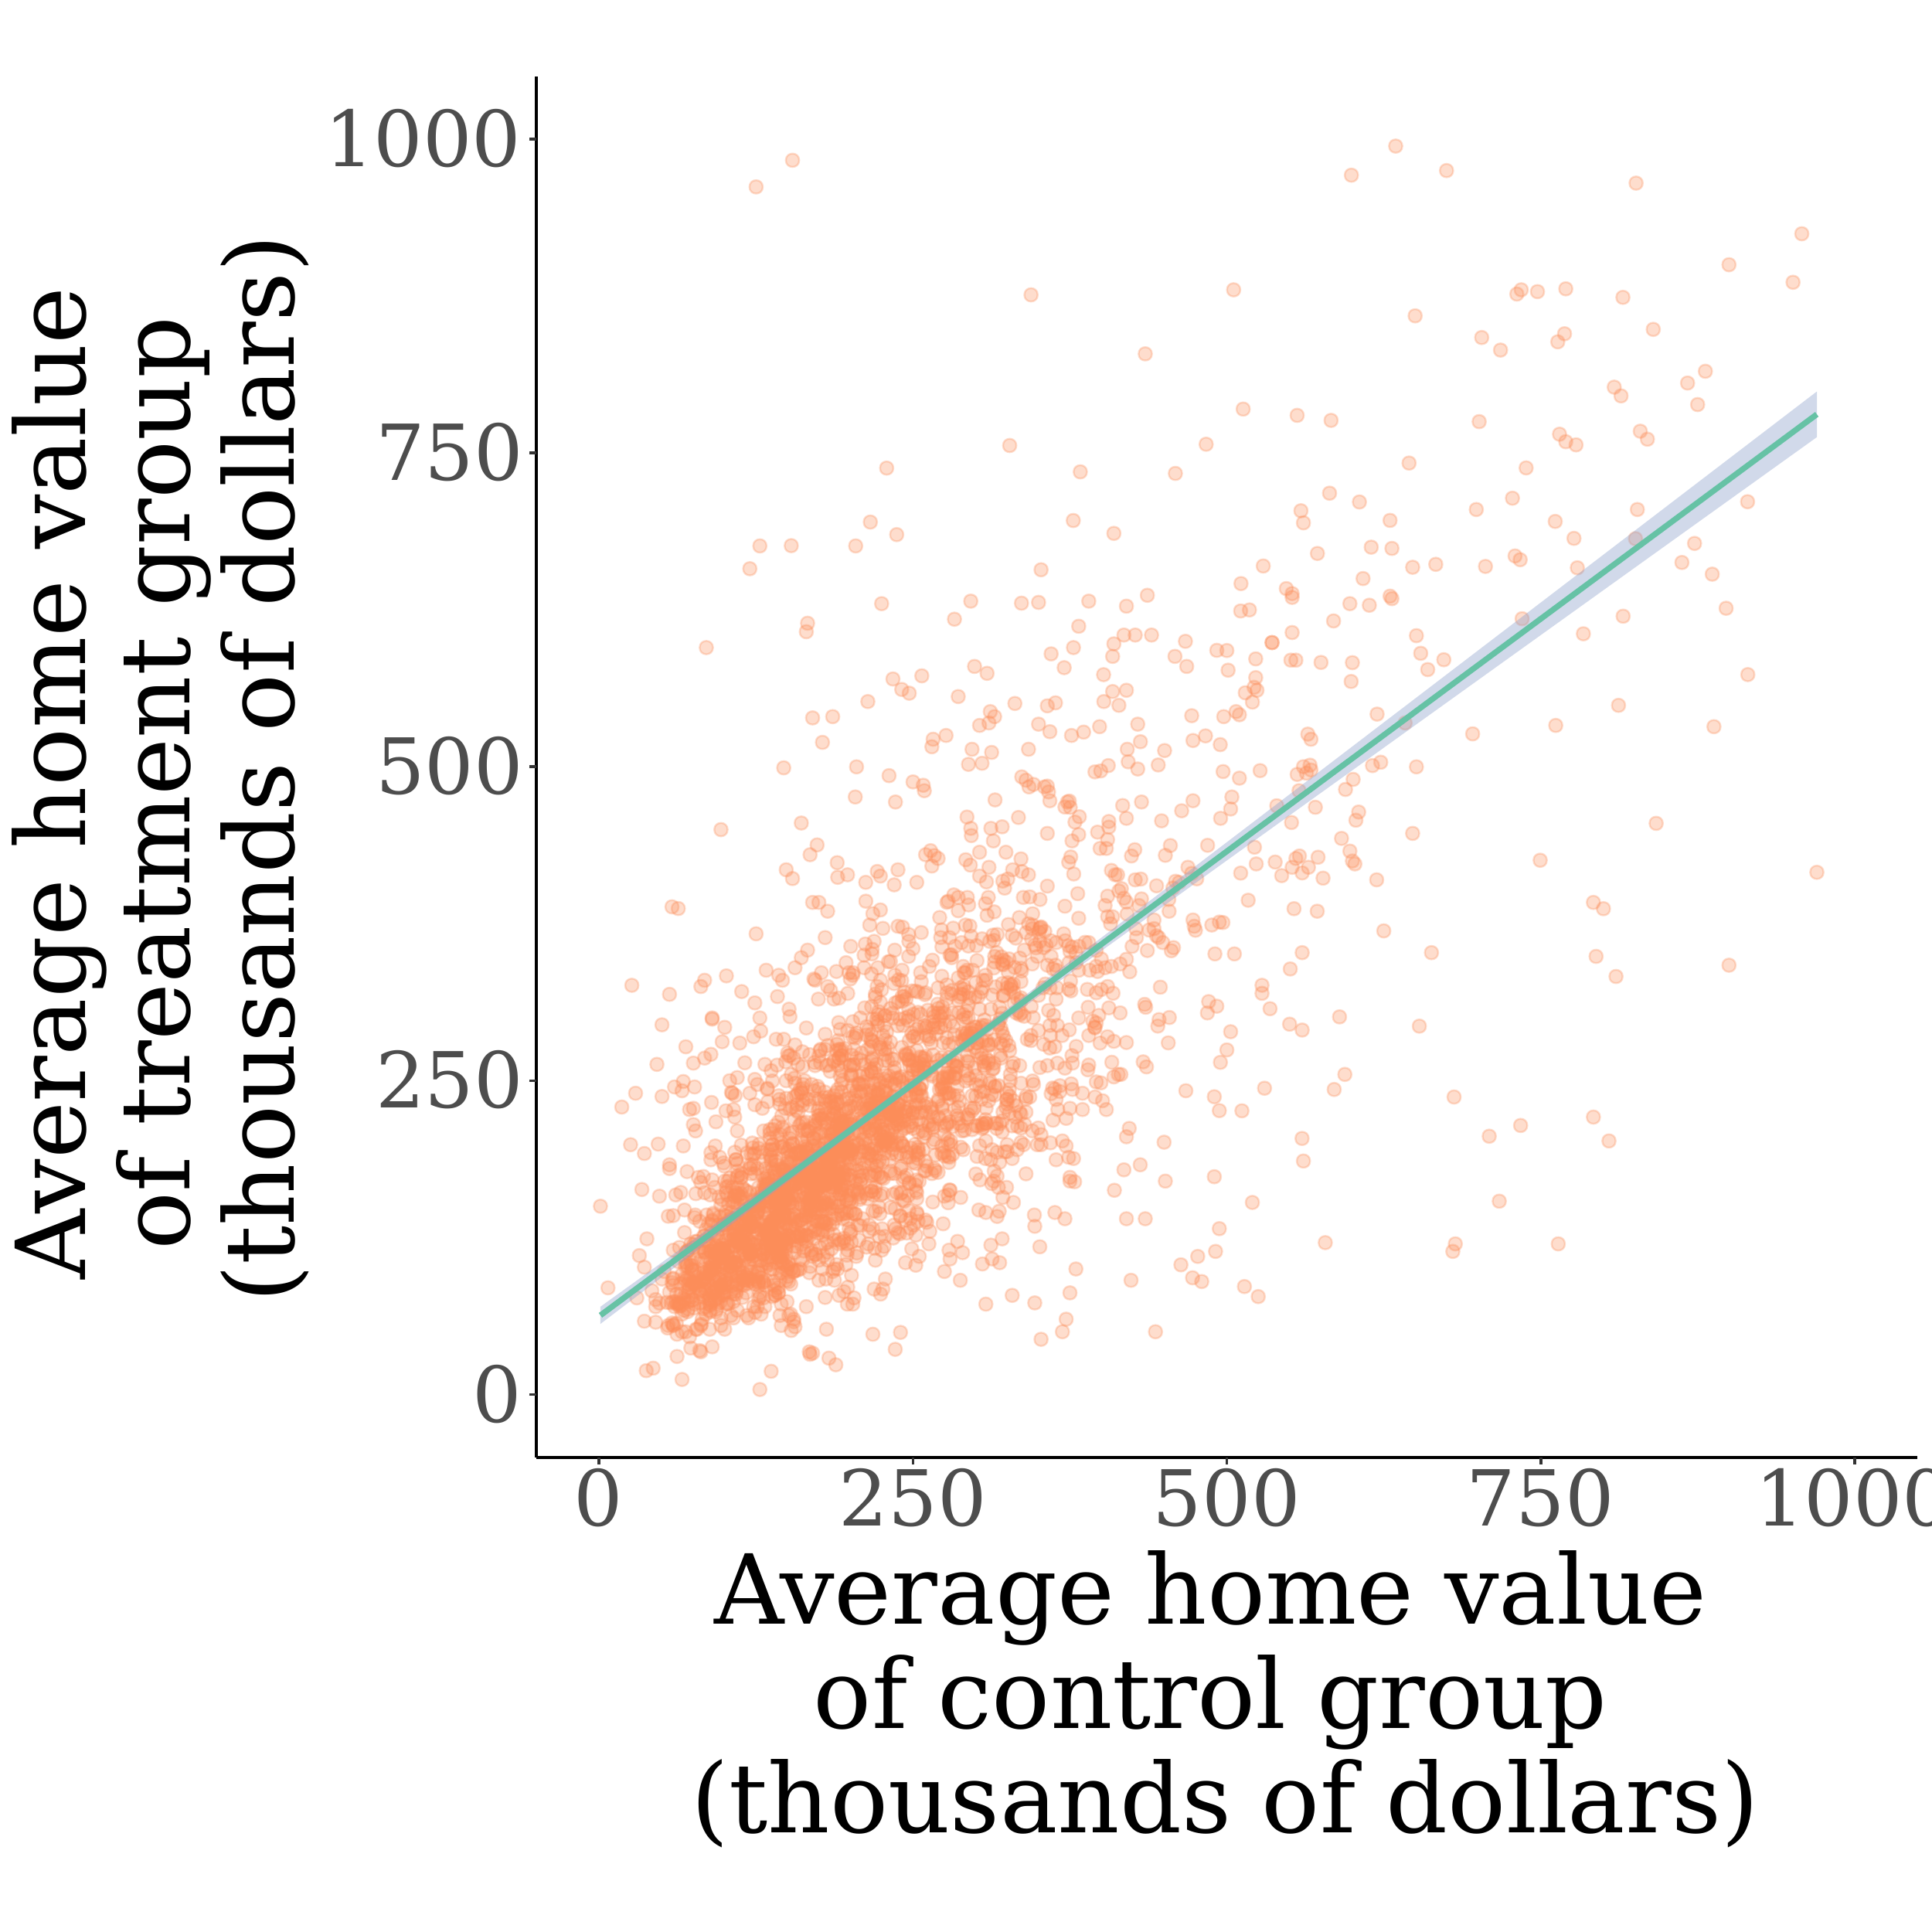}}
    \caption{
   We see that the home prices of \units{} on either block face are similar. (Distance)
    \label{scatter_real_estate_distance}}
\end{figure}

\begin{figure}[H]
\centering
\resizebox{.45\linewidth}{!}{
    \includegraphics[width=.99\columnwidth]{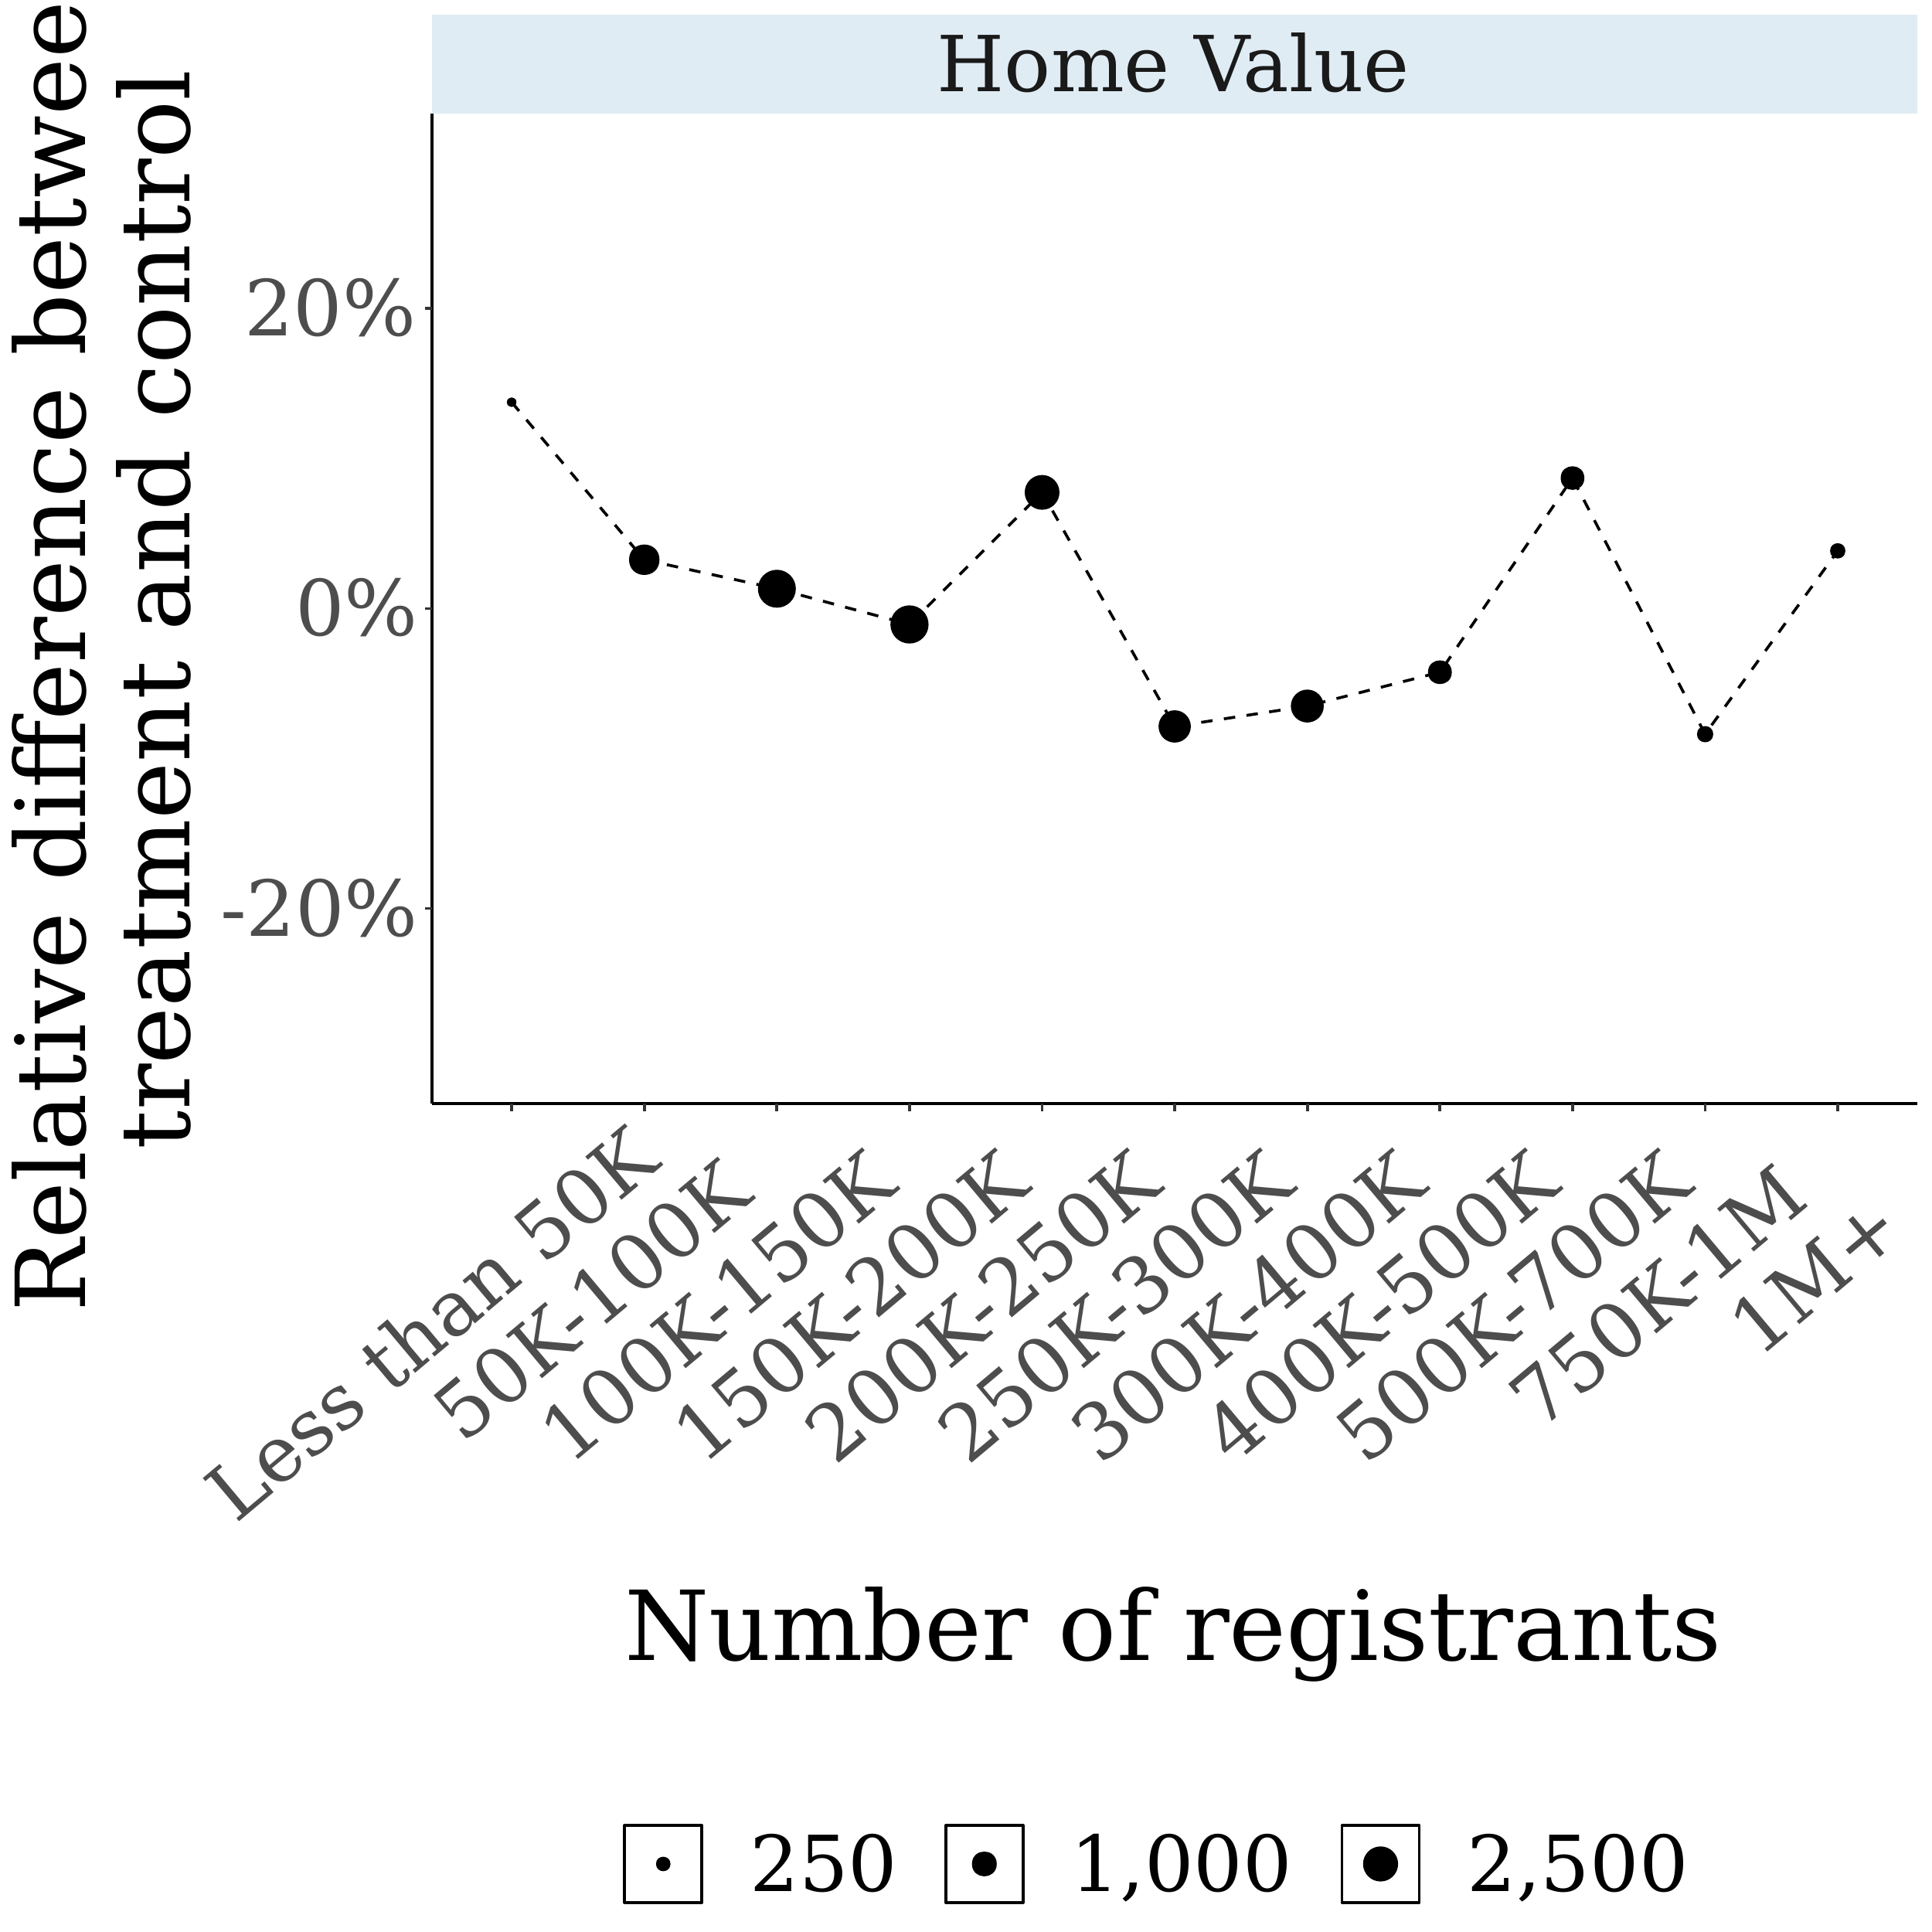}}
    \caption{
   We see that the home prices of \units{} on either block face are similar. (Distance)
    \label{balance_real_estate_distance}}
\end{figure}

\begin{figure}[H]\centering
\resizebox{.7\linewidth}{!}{
    \includegraphics[ width=.99\columnwidth]{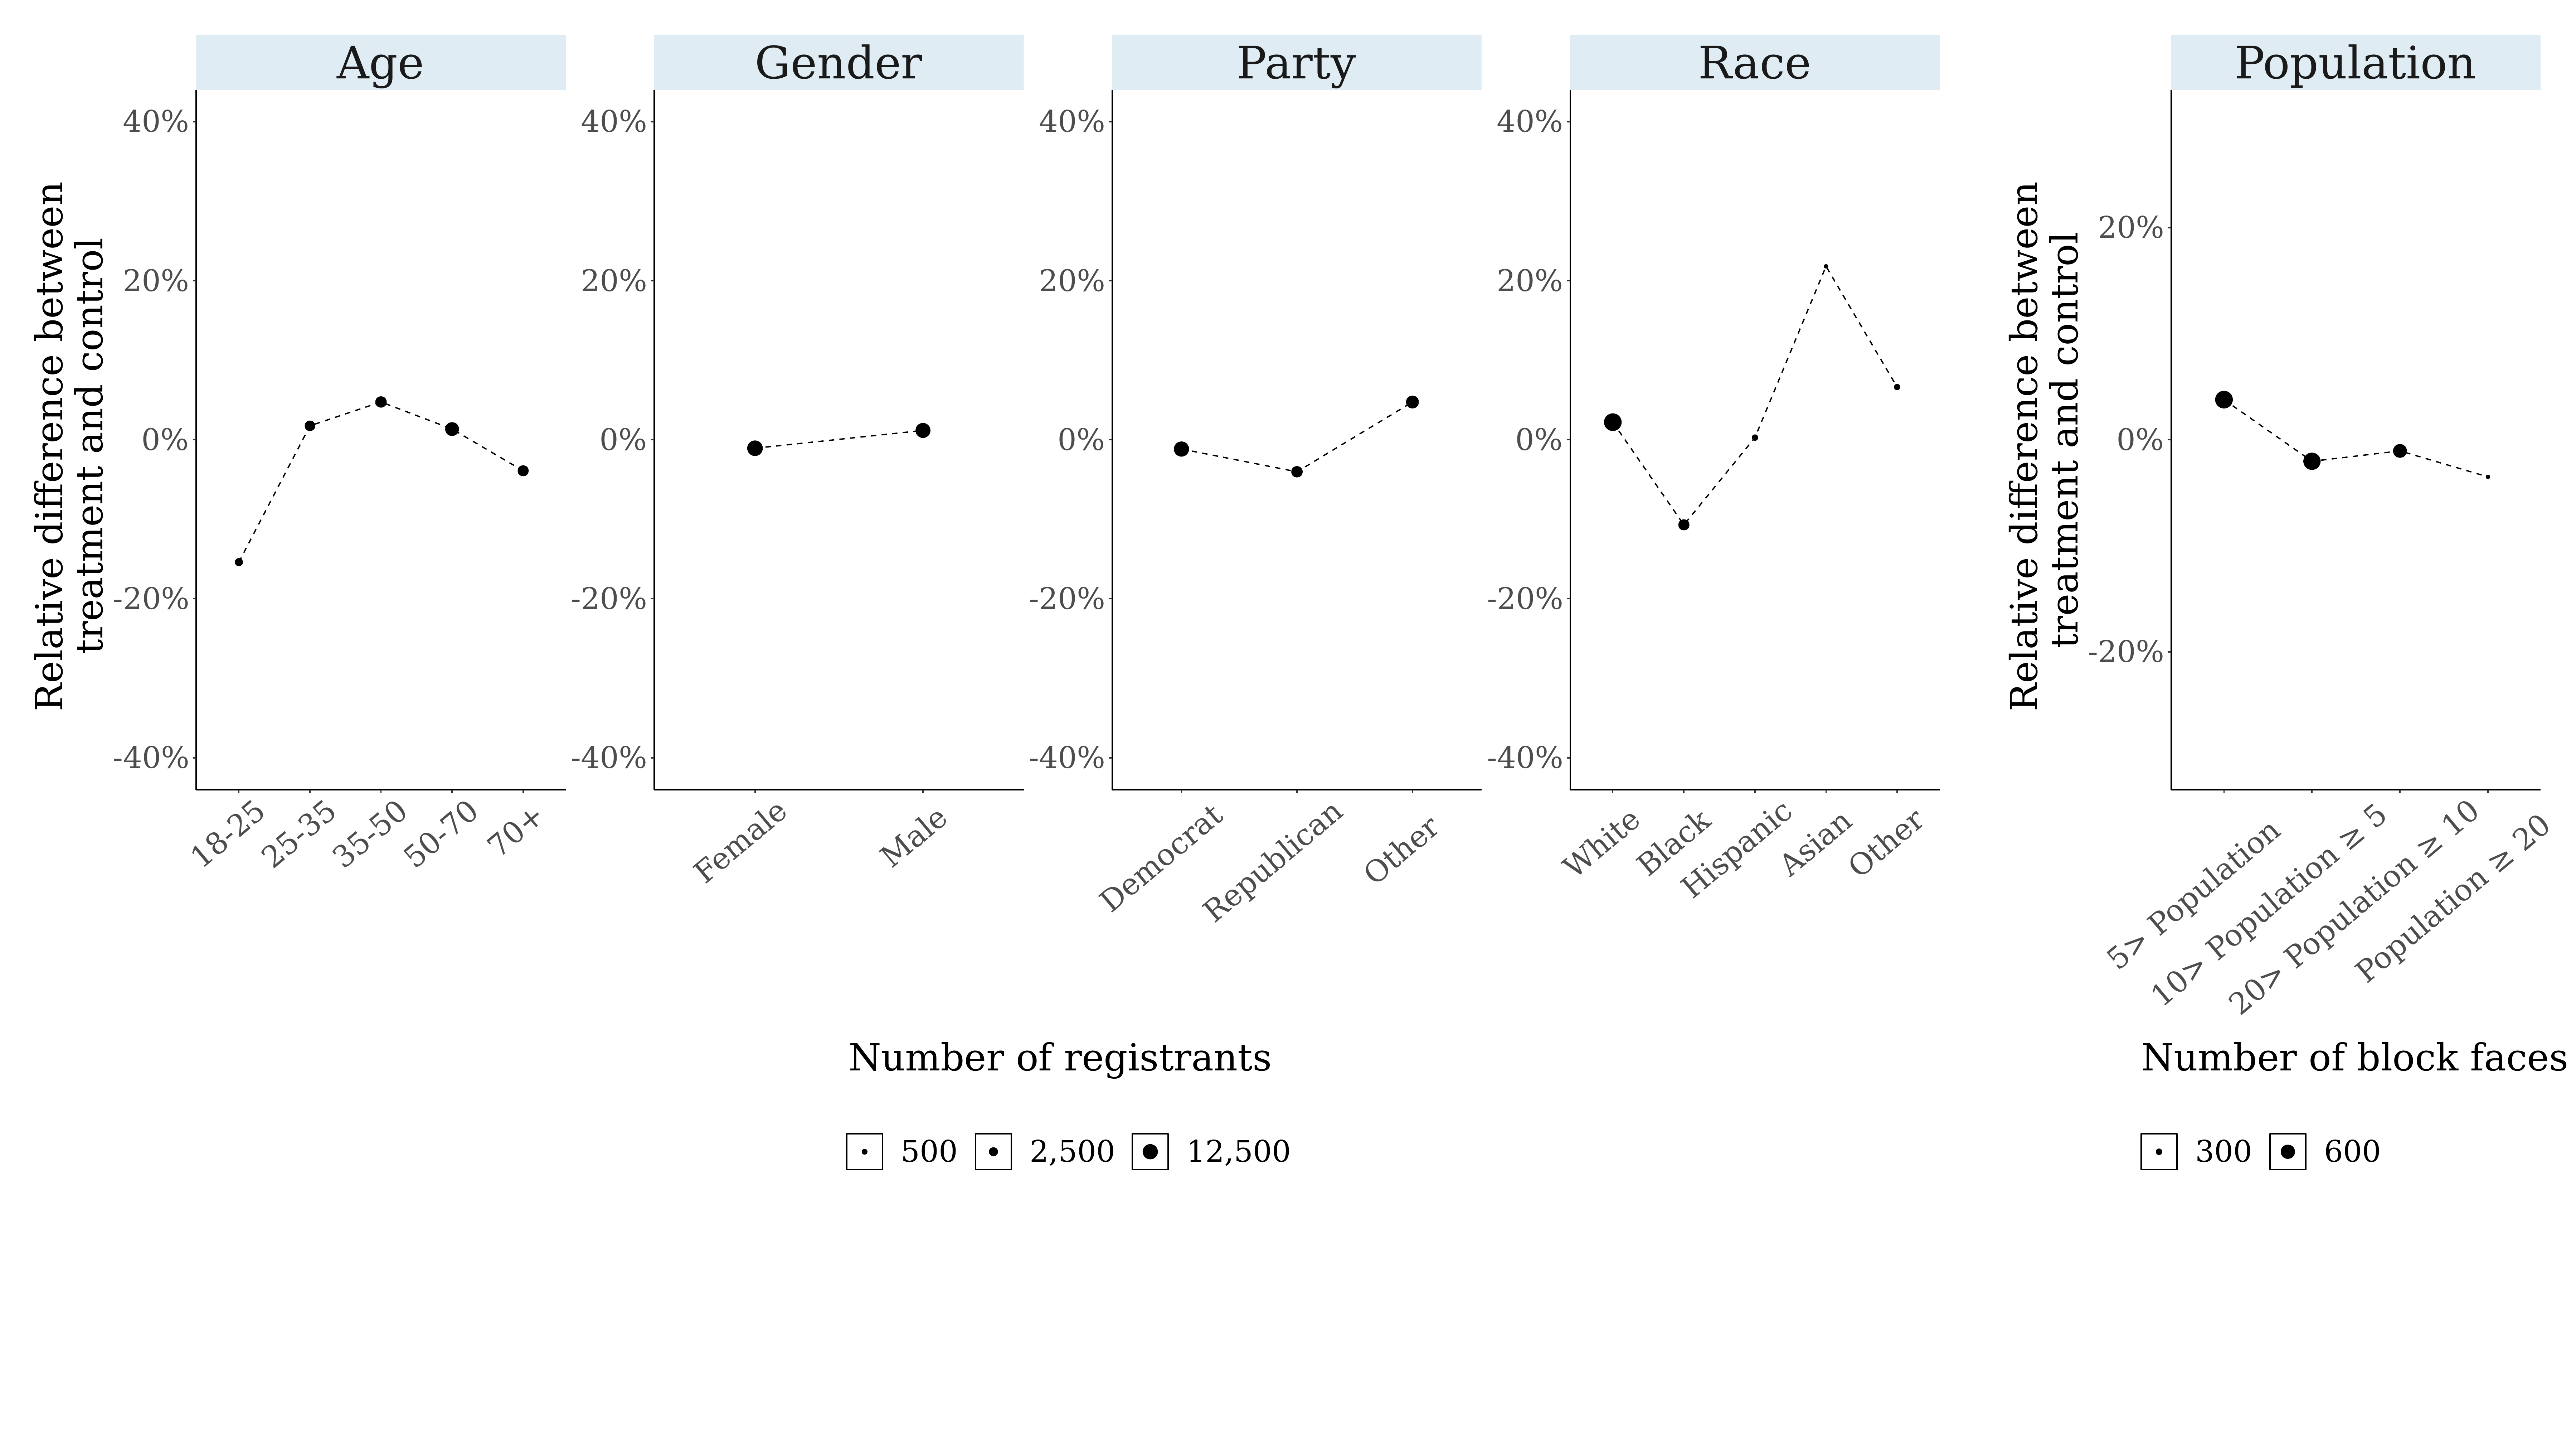}}
    \caption{We see the age, gender, modeled partisanship, modeled race of \units{}, as well as indicators representing that the total number of \units{}, are similar on either block face, although the percent difference can be larger because the sample size is smaller. (Shock)
    } 
    \label{bp_shock}
\end{figure}

\begin{figure}[H]\centering
\resizebox{.4\linewidth}{!}{
    \includegraphics[width=.99\columnwidth]{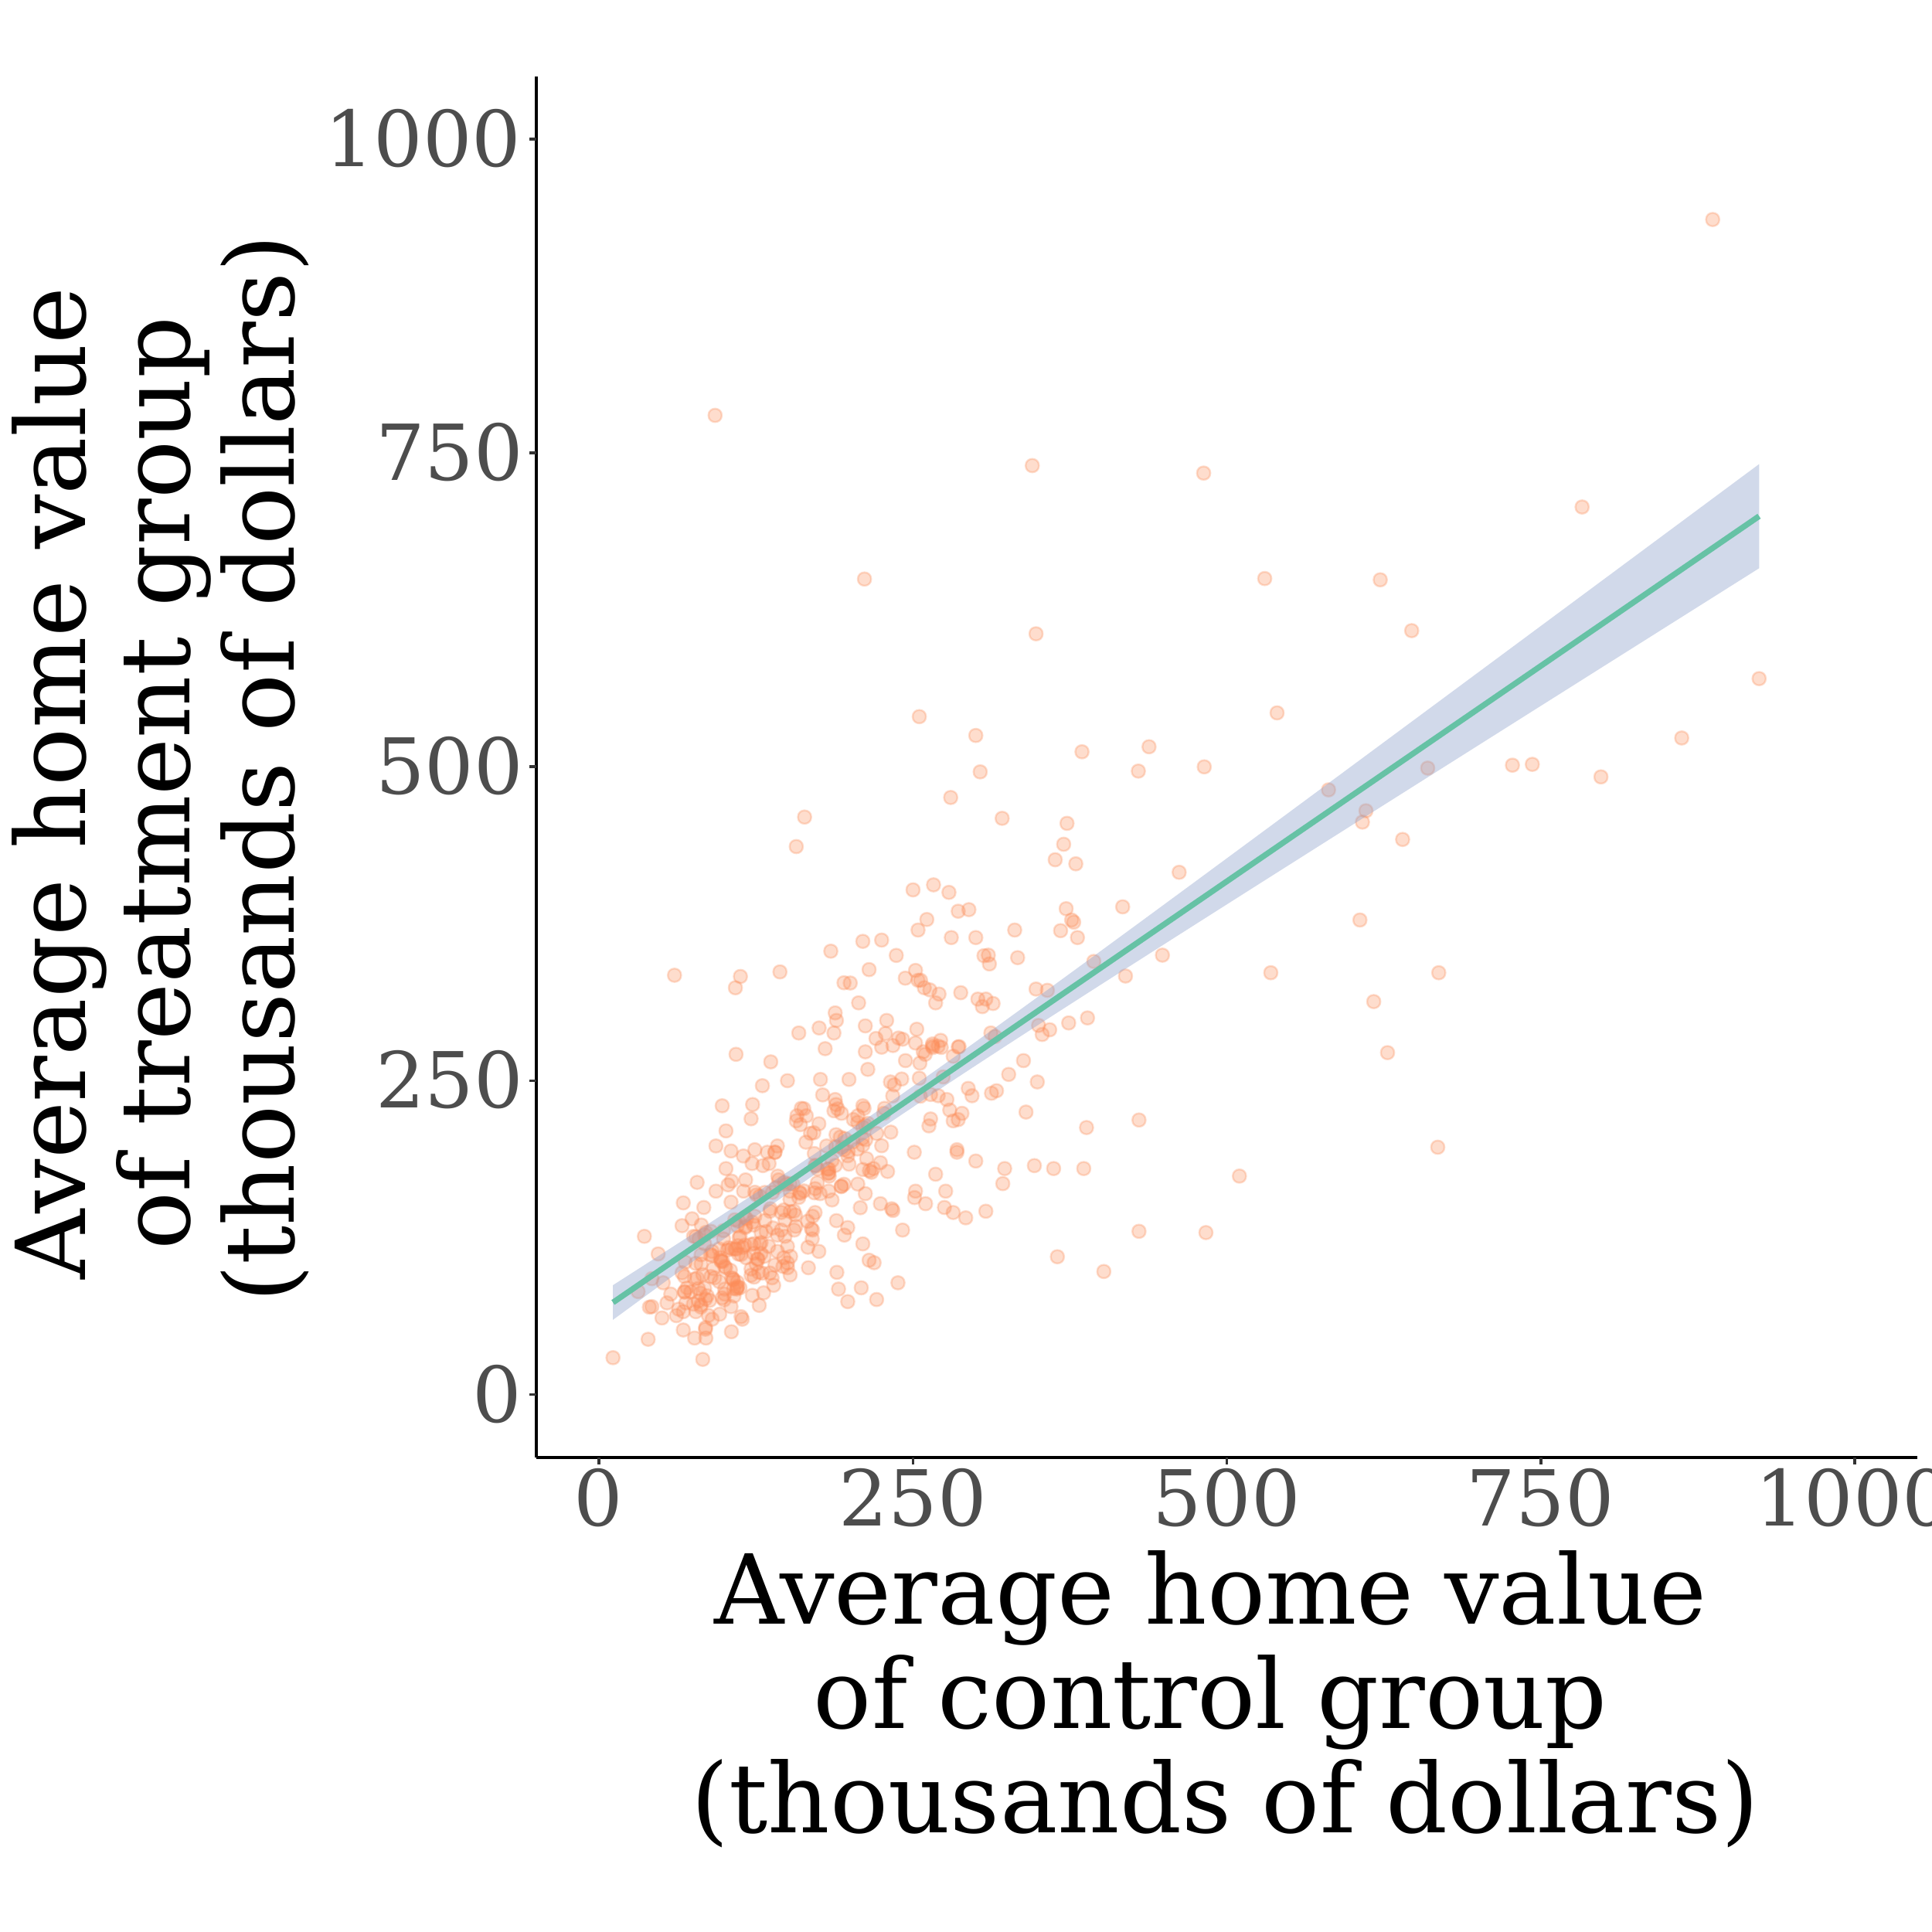}}
    \caption{
   We see that the home prices of \units{} on either block face are similar. (Shock)
    \label{scatter_real_estate_shock}}
\end{figure}

\begin{figure}[H]\centering
\resizebox{.45\linewidth}{!}{
    \includegraphics[width=.99\columnwidth]{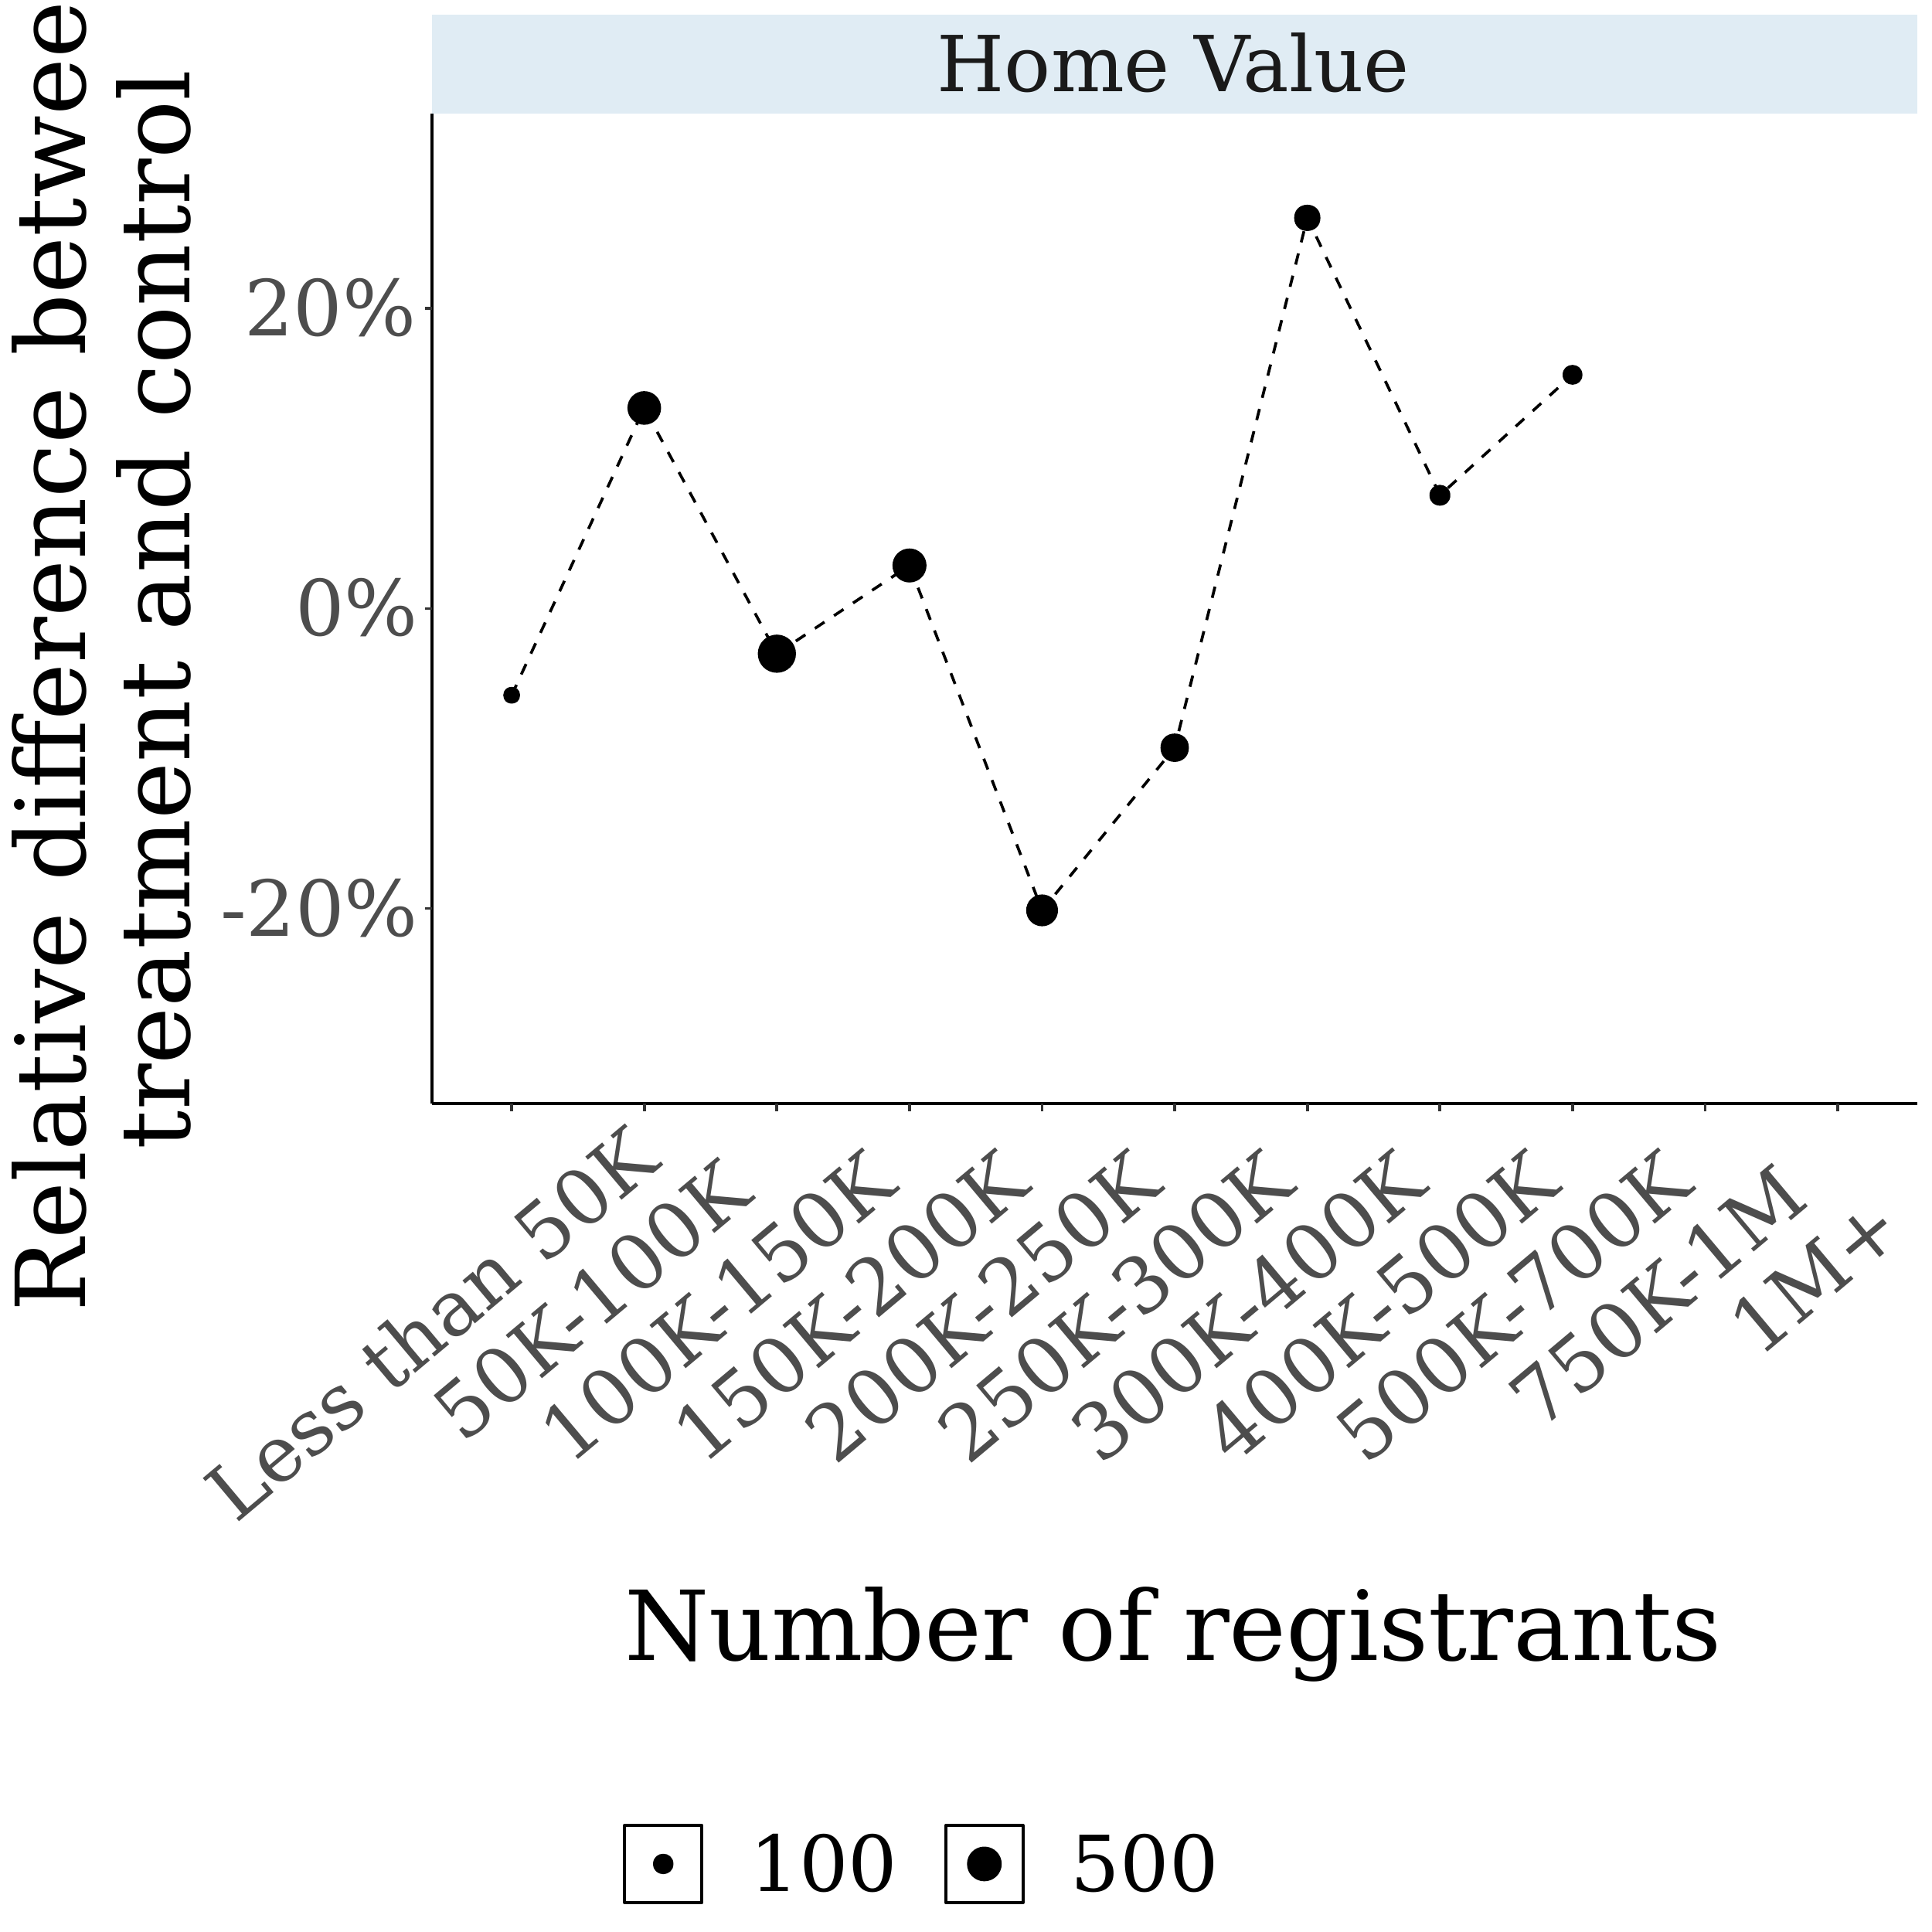}}
    \caption{
   We see that the home prices of \units{} on either block face are similar. (Shock)
    \label{balance_real_estate_shock}}
\end{figure}

\begin{figure}[H]\centering
\resizebox{.45\linewidth}{!}{
    \includegraphics[width=.99\columnwidth]{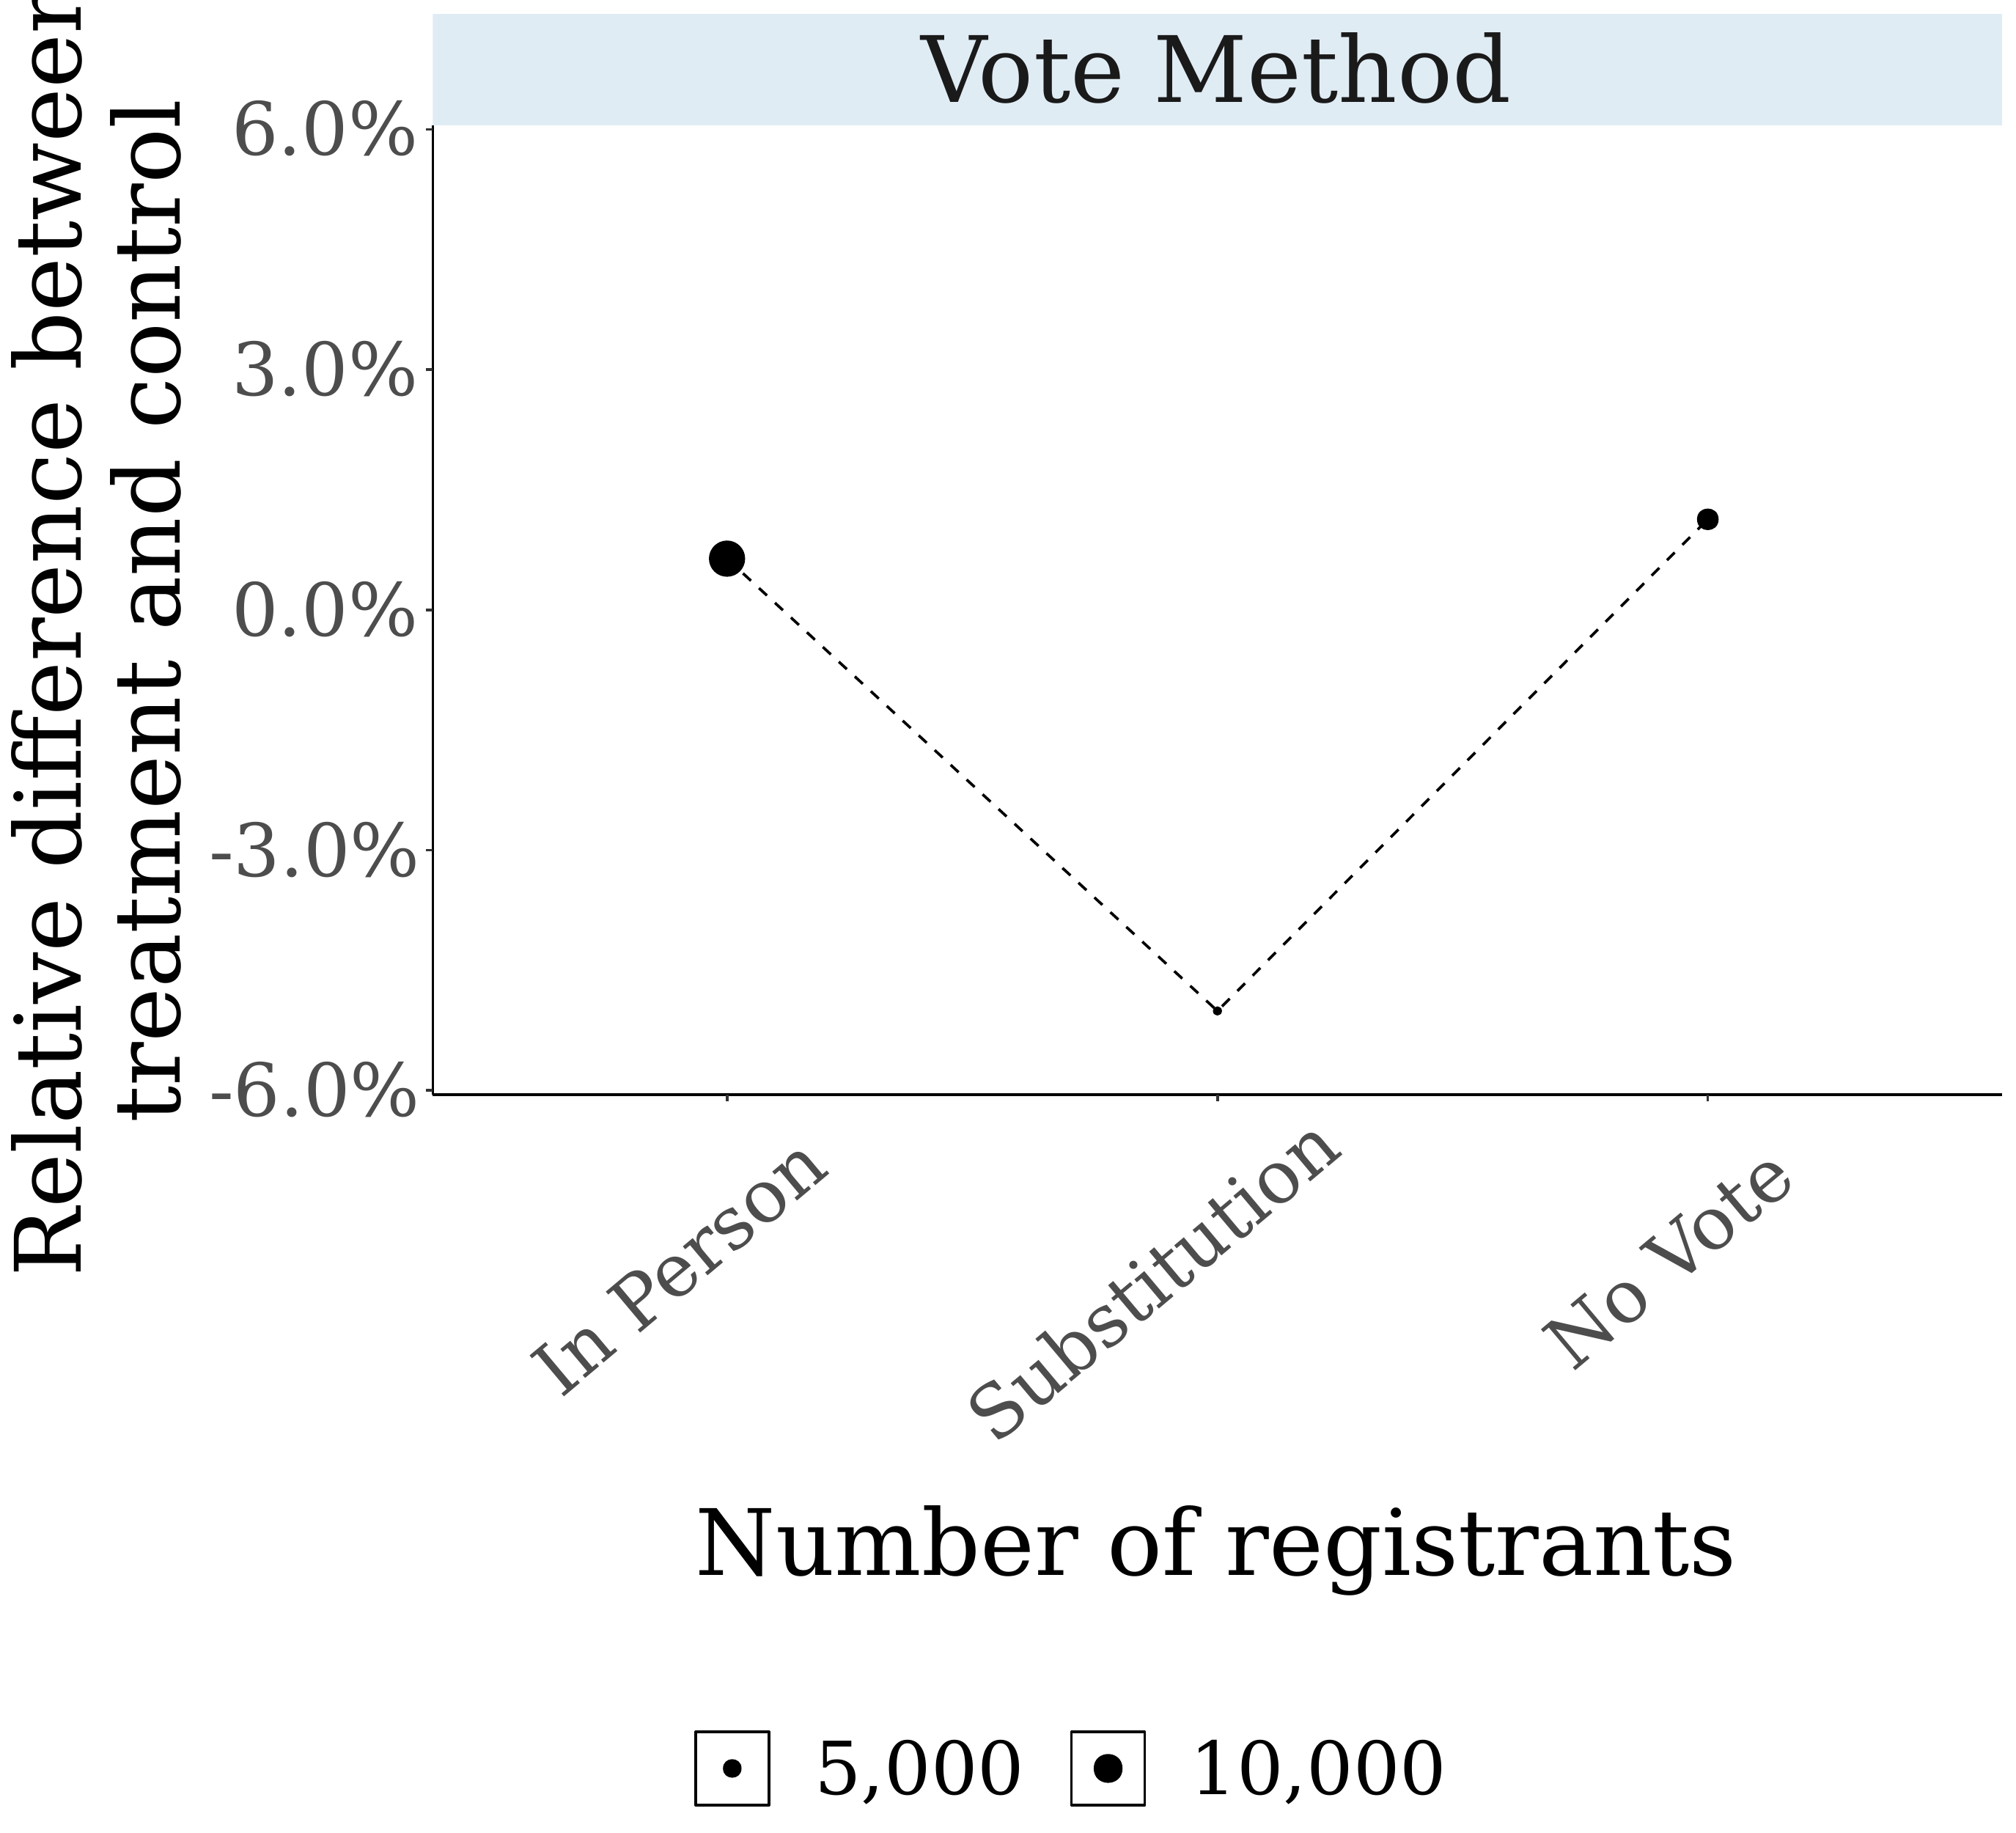}}
    \caption{
   We see that the historical voting patterns in the 2012 presidential election of \units{} on either block face are similar, with \units{} experiencing a shock being, if anything, less likely to vote by substitution than \units{} who did not. The X percent lower usage of substitution voting reflects that Y percent of \units{} who experienced a shock voted using a substitution method in 2012 as compared to Z percent of \units{} who did not.
    \label{balance_past}}
\end{figure}
